# Supplementary material for: Actor-Critic Reinforcement Learning with Simultaneous Human Control and Feedback
Source: arXiv:1703.01274 source file (2017-03-15)
Supplement: Supplementary file 1 [file supplementary.tex]

\onecolumn
\section*{Supplementary Material: Qualitative Feedback from Human Participants}
\begin{itemize}
\item Sometimes I wish that I reacted sooner. Is there a way that I can get the robot to freeze in a current state? I want a way to stop any actions all together unless the EMG control signal changes drastically. I want the system to generalize better. I want to say good boy when it does the right thing, but I know it can not hear me. I want to say STAY and STOP. It is harder when there is a split in the concentration (Control and Feedback condition).
\item It would be easier to relax with a dangle. Is there a timing effect? What if it was more of a simon-says situation, then the human would need to react better and not fall into a pattern. I am attention splitting which is hard on the case when I am doing more than 1 thing (Control and Feedback). 
\item There is a rhythm to just the control case. "Sorry if my timing is off" Am I giving reward to the state of the robot or the state of the robot and action that it last took? Maybe I should decrease the amount of the reward that I am giving to stabilize the learning a bit. I find that I am giving more reward than punishment, because I think that the system has negative covered.
\item Control and Feedback is multitasking. I had to think about it more.  Just matching it is no problem. Just giving reward was easier, then I did not need to remember which one was positive and negative. I wish my arm was more of a direct control signal.
\item How do I get him to stop wiggling? "Make a definitive choice" I am very proud of the robot. Is there a limited number of treats I can give? Just reward feels like a bad video game controller. Why not just use direct control? What if the control space was defined precisely state signal? 
\item I tried to give a little more carrot and a little less stick. I named the robot Carrot McGowan. How do I know if [what the robot is doing] is a good things? Subject was shouting at the robot: "Flex little guy flex! Flex your muscles" and "You really learned!" "Flex Raspberry. Let's go!" He's doing it so much faster now. Why do I reward and punish in twos? 
\item I think that the robot is starting to figure me out. More punishment than feedback. Holding off in the beginning. Is there a way to give continual reward? I am building an internal model of the value of certain things, and I am changing it based on the assumed value of certain things (reward, state). Am I giving coarse or hyper specific training? 
\item Subject was talking to robot "Terrible, you are killing me here", "Good", "Very good", "You are doing bad now", " You, that is really good", "I am only giving you good reward". Did the reward really affect the learning? I want to see what the robot sees, all the signals.
\item "Why do you keep going out, out is bad". Whispering to the robot "bad", "very bad", "come on FLEX". Easier to flex than to relax. I am surprised how well it learns how to perform the task. It is unclear if you are rewarding the state or the direction it is moving in. "I think I messed you up little guy". It is easier to just give reward rather than reward and punishment. Late punishment seems to confuse the robot. It is confusing to do both control and feedback at once.
\item Talking to the robot: "now you are switching", "do the thing now", "Okay, I will give you a bit now that you are going the right direction.", "yes, no, maybe!". Not convinced that the reward actually mattered. Reward and punishment gave no clear, immediate impact. Maybe by the end it was learning what I really meant. 
\item When controlling and providing feedback I was waiting to see if it would do something right before I will reward it. Shifted to only reward near the end, maybe because it was doing all the right things, and maybe because it hit a performance ceiling.
\item It is very satisfying to give reward. It is nice to understand that the learning is happening and it feels good to work together.  Is there a way that the robot can fall into a reward trap? Often times I was punishing for the lack of evidence of future intention. I felt limited by the perception of the robot from the viewing angle, I wanted to see more signals. More information would make the task easier. "I want to see what the robot really values". A joystick could provide non-linear reward. Directly controlling or nudging the robot to the right direction. Subject was curious about if there was a budget for the feedback or not.
\end{itemize}
